# Supplementary material for: Entangled massive mechanical oscillators
Source: arXiv:1711.01640 ancillary file (2017-11-05)
Supplement: Supplementary file 1 [file EntanglementSupplArxiv.pdf]

# Entangled massive mechanical oscillators: Supplementary Information

C. F. Ockeloen-Korppi,[1] E. Damskägg,[1] J.-M. Pirkkalainen,[1] A. A. Clerk,[2] F. Massel,[3] M. J. Woolley,[4] and M. A. Sillanpää[1, *]

[1] *Department of Applied Physics, Aalto University, P.O. Box 15100, FI-00076 AALTO, Finland*
[2] *Institute for Molecular Engineering, University of Chicago, Chicago, IL, 60631, USA*
[3] *Department of Physics and Nanoscience Center, University of Jyväskylä, P.O. Box 35 (YFL), FI-40014 University of Jyväskylä, Finland*
[4] *School of Engineering and Information Technology, UNSW Canberra, ACT, 2600, Australia*

## CONTENTS

I. Theoretical description 1
A. Hamiltonian under two-tone driving 1
B. Hamiltonian under four-tone driving 3
C. Heisenberg-Langevin equations 5
D. Noise spectra 6

II. Experimental calibrations 8
A. Probe spectrum 8
1. Thermal state of the mechanics 8
B. Thermal calibrations 9
C. Power calibration of BAE signal 10
D. Effective couplings of the probes 11
E. Effective couplings of the pumps 12
F. Additional data and list of parameters 12

III. Error analysis 15
A. Probe spectra 15
B. Pump spectra 15
C. Ratio of quadrature variances 17

References 17

## I. THEORETICAL DESCRIPTION

### A. Hamiltonian under two-tone driving

The Hamiltonian describing two mechanical oscillators coupled to a common microwave cavity by radiation-pressure-like couplings is [1]

$$\hat{H} = \omega_c \hat{a}^\dagger \hat{a} + \omega_1 \hat{b}_1^\dagger \hat{b}_1 + \omega_2 \hat{b}_2^\dagger \hat{b}_2 + g_1(\hat{b}_1 + \hat{b}_1^\dagger)\hat{a}^\dagger \hat{a} + g_2(\hat{b}_2 + \hat{b}_2^\dagger)\hat{a}^\dagger \hat{a} + \hat{H}_{\text{drive}}, \tag{S1}$$

where $\omega_c$, $\omega_1$, and $\omega_2$ denote the resonance frequencies of the microwave cavity and mechanical oscillator modes (respectively), $\hat{a}$, $\hat{b}_1$, and $\hat{b}_2$ denote the corresponding annihilation operators, and $g_1$ and $g_2$ are the single-photon optomechanical coupling rates between the mechanical oscillators and the cavity. Two-tone driving of the cavity mode is described by [2–4]

$$\hat{H}_{\text{drive}} = \left(\mathcal{E}_+^* e^{i\omega_+ t} + \mathcal{E}_-^* e^{i\omega_- t}\right)\hat{a} + \text{H.c.}, \tag{S2}$$

* mika.sillanpaa@aalto.fi

where $\omega_\pm$ denote the driving frequencies, detuned by $\delta_\pm$ from the mechanical sidebands either side of the cavity resonance frequency (see Fig. 1 of the main text) and so given by

$$\omega_+ = \omega_c + \omega_2 + \delta_+ \,, \tag{S3a}$$
$$\omega_- = \omega_c - \omega_1 + \delta_- \,. \tag{S3b}$$

For the purpose of further analysis, it is useful to work with an interaction picture Hamiltonian, given by $\hat{H}_I = \hat{U}_0^\dagger \hat{H} \hat{U}_0 - i\hbar \hat{U}_0^\dagger \frac{\partial \hat{U}_0}{\partial t}$ where $\hat{U}_0 = \exp(-i\hat{H}_0 t/\hbar)$ with [3, 4]

$$\hat{H}_0 = \left(\omega_c + \Omega + \bar{\delta}\right) \hat{a}^\dagger \hat{a} + (\bar{\omega} + \Delta)\left(\hat{b}_1^\dagger \hat{b}_1 + \hat{b}_2^\dagger \hat{b}_2\right). \tag{S4}$$

In Eq. (S4) we have introduced notation for the average and half-difference of the mechanical resonance frequencies,

$$\bar{\omega} = \frac{\omega_1 + \omega_2}{2}, \tag{S5a}$$
$$\Omega = \frac{\omega_2 - \omega_1}{2}, \tag{S5b}$$

respectively, and for the average and half-difference of the cavity driving tone detunings,

$$\bar{\delta} = \frac{\delta_+ + \delta_-}{2}, \tag{S6a}$$
$$\Delta = \frac{\delta_+ - \delta_-}{2}, \tag{S6b}$$

respectively. The result of this transformation is the interaction picture Hamiltonian,

$$\begin{aligned}\hat{H}_I = &-\left(\Omega + \bar{\delta}\right)\hat{a}^\dagger \hat{a} + \Omega\left(\hat{b}_2^\dagger \hat{b}_2 - \hat{b}_1^\dagger \hat{b}_1\right) - \Delta\left(\hat{b}_1^\dagger \hat{b}_1 + \hat{b}_2^\dagger \hat{b}_2\right) \\ &+ g_1\left[\hat{b}_1 e^{-i(\bar{\omega}+\Delta)t} + \hat{b}_1^\dagger e^{+i(\bar{\omega}+\Delta)t}\right]\hat{a}^\dagger \hat{a} + g_2\left[\hat{b}_2 e^{-i(\bar{\omega}+\Delta)t} + \hat{b}_2^\dagger e^{+i(\bar{\omega}+\Delta)t}\right]\hat{a}^\dagger \hat{a} \\ &+ \left[\left(\mathcal{E}_+^* e^{+i(\bar{\omega}+\Delta)t} + \mathcal{E}_-^* e^{-i(\bar{\omega}+\Delta)t}\right)\hat{a} + \text{H.c.}\right].\end{aligned} \tag{S7}$$

Note that in the absence of detunings from the cavity's mechanical sidebands (i.e., $\delta_\pm = 0$ such that $\Delta = 0$), the Hamiltonian Eq. (S4) corresponds to a transformation into a frame rotating at the average of the mechanical resonance frequencies.

The quantity $\bar{\delta}$ in Eq. (S6a) indicates how much the pump centre frequency is shifted from the nominal case (both mechanics pumped at sidebands); that is, $\bar{\delta} = 0$. Generally, the physics is very insensitive to non-zero $\bar{\delta}$. In the original proposal of Ref. [4], $\bar{\delta} = -\Omega = -\frac{\omega_2 - \omega_1}{2}$ and basically $\bar{\delta}$ can be varied between that value and slightly above zero with very similar anticipated levels of entanglement. On the contrary, the other detuning $\Delta$ in Eq. (S6b) very sensitively affects the performance of the entangling protocol. Nominally, $\Delta = 0$, which is the optimum case in a situation fully symmetric with respect to couplings and damping rates. However, as mentioned in the main text, we find numerically that introducing $\Delta$ of the order several mechanical linewidths can compensate (in some cases overcompensate) for asymmetries.

The Heisenberg-Langevin equations corresponding to the Hamiltonian Eq. (S7), including damping of the cavity and mechanical oscillator modes into independent thermal baths, are

$$\begin{aligned}\dot{\hat{a}} = &+i(\Omega + \bar{\delta})\hat{a} - ig_1\left[\hat{b}_1 e^{-i(\bar{\omega}+\Delta)t} + \hat{b}_1^\dagger e^{+i(\bar{\omega}+\Delta)t}\right]\hat{a} - ig_2\left[\hat{b}_2 e^{-i(\bar{\omega}+\Delta)t} + \hat{b}_2^\dagger e^{+i(\bar{\omega}+\Delta)t}\right]\hat{a} \\ &-i\mathcal{E}_+ e^{-i(\bar{\omega}+\Delta)t} - i\mathcal{E}_- e^{+i(\bar{\omega}+\Delta)t} - \frac{\kappa}{2}\hat{a} + \sqrt{\kappa_E}\hat{a}_E^{\text{in}} + \sqrt{\kappa_I}\hat{a}_I^{\text{in}},\end{aligned} \tag{S8a}$$
$$\dot{\hat{b}}_1 = -i(\Omega - \Delta)\hat{b}_1 - ig_1 \hat{a}^\dagger \hat{a} e^{i(\bar{\omega}+\Delta)t} - \frac{\gamma_1}{2}\hat{b}_1 + \sqrt{\gamma_1}\hat{b}_1^{\text{in}}, \tag{S8b}$$
$$\dot{\hat{b}}_2 = +i(\Omega + \Delta)\hat{b}_2 - ig_2 \hat{a}^\dagger \hat{a} e^{i(\bar{\omega}+\Delta)t} - \frac{\gamma_2}{2}\hat{b}_2 + \sqrt{\gamma_2}\hat{b}_2^{\text{in}}, \tag{S8c}$$

where $\kappa = \kappa_I + \kappa_E$ is the sum of the internal and external cavity damping rates, and $\gamma_1$ and $\gamma_2$ are the mechanical oscillator damping rates.

Substituting the ansatz $\hat{a}(t) = \hat{a}_0(t) + \hat{a}_+(t)e^{-i(\bar{\omega}+\Delta)t} + \hat{a}_-(t)e^{+i(\bar{\omega}+\Delta)t}$ into Eqs. (S8a)-(S8c), separating frequency components, making a rotating-wave approximation, and solving for the steady-state at the driven sidebands leads to

the amplitudes [5]

$$\langle \hat{a}_+ \rangle = \frac{i\mathcal{E}_+}{+i(\omega_1 + \delta_+) - \kappa/2} \equiv \alpha_+ e^{i\psi_+}, \tag{S9a}$$

$$\langle \hat{a}_- \rangle = \frac{i\mathcal{E}_-}{-i(\omega_2 - \delta_-) - \kappa/2} \equiv \alpha_- e^{i\psi_-}. \tag{S9b}$$

Substituting these amplitudes into Eqs. (S8a)-(S8c) we find that the system may be described by the time-independent effective Hamiltonian,

$$\begin{aligned}\hat{H}_\mathrm{I} =& -\left(\Omega + \bar{\delta}\right) \hat{a}^\dagger \hat{a} + \Omega \left(\hat{b}_2^\dagger \hat{b}_2 - \hat{b}_1^\dagger \hat{b}_1\right) - \Delta \left(\hat{b}_1^\dagger \hat{b}_1 + \hat{b}_2^\dagger \hat{b}_2\right) \\ &+ \left(g_1 \alpha_- e^{i\psi_-} \hat{a}^\dagger \hat{b}_1 + g_1 \alpha_+ e^{i\psi_+} \hat{a}^\dagger \hat{b}_1^\dagger + g_2 \alpha_- e^{i\psi_-} \hat{a}^\dagger \hat{b}_2 + g_2 \alpha_+ e^{i\psi_+} \hat{a}^\dagger \hat{b}_2^\dagger + \mathrm{H.c.}\right). \end{aligned} \tag{S10}$$

Without the rotating-wave approximation, the Hamiltonian in Eq. (S10) would have additional (explicitly time-dependent) contributions such that $\hat{H}_\mathrm{I}(t) = \hat{H}_\mathrm{I} + \hat{H}_\mathrm{rot}(t)$ where

$$\hat{H}_\mathrm{rot}(t) = g_1 \alpha_- a^\dagger b_1 \exp(-2i\bar{\omega}t) + g_2 \alpha_+ a^\dagger b_2 \exp(-2i\bar{\omega}t) + g_1 \alpha_-^* a b_1 \exp(-2i\bar{\omega}t) + g_2 \alpha_-^* a b_2 \exp(-2i\bar{\omega}t) + \mathrm{H.c.} \tag{S11}$$

In all the modeling henceforth, we shall neglect this fast-rotating contribution. This is justified because the terms are rotating at a relatively fast frequency $2\bar{\omega}$ that is approximately twice the mechanical frequencies. Since we are deep in the resolved sideband regime, $\kappa \ll \omega_{1,2}$, the off-resonant terms are fully suppressed by the cavity response, see Ref. [4].

The possibility of using the Hamiltonian in Eq. (S10) to entangle the mechanical oscillators is seen more clearly if we rewrite Eq. (S10) in terms of two-mode Bogoliubov operators [4]. For the sake of clarity here, we first make the simplifying assumptions $\psi_\pm = 0$, $g_1 = g_2 \equiv g$, and $\Delta = 0$ in Eq. (S10), and then introduce effective optomechanical coupling rates $G_\pm = g\alpha_\pm$. Explicitly, we define the two-mode Bogoliubov operators,

$$\hat{\beta}_1 = \hat{b}_1 \cosh r + \hat{b}_2^\dagger \sinh r, \tag{S12a}$$

$$\hat{\beta}_2 = \hat{b}_2 \cosh r + \hat{b}_1^\dagger \sinh r, \tag{S12b}$$

where the parameter $r$ is defined by the relationship

$$\tanh r = \frac{G_+}{G_-}. \tag{S13}$$

The (entangled) two-mode squeezed state is the simultaneous eigenstate corresponding to the zero eigenvalue of the operators $\hat{\beta}_1$ and $\hat{\beta}_2$. Now Eq. (S13) allows us to write $G_- = \mathcal{G}\sinh r$ and $G_+ = \mathcal{G}\cosh r$, leading to the identification

$$\mathcal{G} = \sqrt{G_-^2 - G_-^2}, \tag{S14}$$

and the Hamiltonian Eq. (S10) may be rewritten as

$$\hat{H}_\mathrm{I} = -(\Omega + \bar{\delta})\hat{a}^\dagger \hat{a} + \Omega\left(\hat{\beta}_2^\dagger \hat{\beta}_2 - \hat{\beta}_1^\dagger \hat{\beta}_1\right) + \mathcal{G}\left[\hat{a}^\dagger \left(\hat{\beta}_1 + \hat{\beta}_2\right) + \hat{a}\left(\hat{\beta}_1^\dagger + \hat{\beta}_2^\dagger\right)\right], \tag{S15}$$

as per Eq. (1) of the Main Text. As shown in Ref. [4], this Hamiltonian can result in the preparation of a two-mode squeezed state of the mechanical oscillators. The cavity cools the sum of the Bogoliubov modes, and the all-mechanical part of Eq. (S15) couples the difference of the Bogoliubov modes to the sum of the Bogoliubov modes, which is equivalent to cooling to the ground state of both Bogoliubov modes, corresponding to the preparation of a two-mode squeezed state.

### B. Hamiltonian under four-tone driving

In practice, two driving tones are used to prepare the two-mode squeezed state (henceforth, the *pump* tones), while two other driving tones are used to measure the state prepared (henceforth, the *probe* tones). Ideally, the pump tones (denoted $\omega_\pm$ as above) are applied at the mechanical sidebands corresponding to $\delta_\pm = 0$ [2, 4], and the probe tones (henceforth denoted by $\omega_{\mathrm{d}\pm}$, the d subscript indicating that these tones are responsible for detection) are applied in between the mechanical sidebands corresponding to $\delta_\pm = -\Omega$ [3, 6]. Therefore, the pump and probe tones are

well-resolved in frequency space and may be treated as effectively independent modes, $\hat{a}$ and $\hat{a}_{\rm d}$, with steady-state coherent amplitudes $\alpha_\pm e^{i\psi_\pm}$ and $\alpha^{\rm d}_\pm e^{\pm i\phi}$, respectively. Accordingly, the effective Hamiltonian in this case is

$$\begin{aligned}\hat{H}_I = &-\left(\Omega+\bar{\delta}\right)\hat{a}^\dagger\hat{a} - \left(\Omega+\bar{\delta}_{\rm d}\right)\hat{a}^\dagger_{\rm d}\hat{a}_{\rm d} + \Omega\left(\hat{b}^\dagger_2\hat{b}_2 - \hat{b}^\dagger_1\hat{b}_1\right) - \Delta\left(\hat{b}^\dagger_1\hat{b}_1 + \hat{b}^\dagger_2\hat{b}_2\right)\\ &+\left(g_1\alpha_- e^{i\psi_-}\hat{a}^\dagger\hat{b}_1 + g_1\alpha_+ e^{i\psi_+}\hat{a}^\dagger\hat{b}^\dagger_1 + g_2\alpha_- e^{i\psi_-}\hat{a}^\dagger\hat{b}_2 + g_2\alpha_+ e^{i\psi_+}\hat{a}^\dagger\hat{b}^\dagger_2 + \text{H.c.}\right)\\ &+\left(g_1\alpha^{\rm d}_- e^{-i\phi}\hat{a}^\dagger_{\rm d}\hat{b}_1 + g_1\alpha^{\rm d}_+ e^{+i\phi}\hat{a}^\dagger_{\rm d}\hat{b}^\dagger_1 + g_2\alpha^{\rm d}_- e^{-i\phi}\hat{a}^\dagger_{\rm d}\hat{b}_2 + g_2\alpha^{\rm d}_+ e^{+i\phi}\hat{a}^\dagger_{\rm d}\hat{b}^\dagger_2 + \text{H.c.}\right),\end{aligned} \tag{S16}$$

where we have imposed the constraint $\Delta_{\rm d} = \Delta$ (that is, the frequency spacing between the two pump tones is the same as the frequency spacing between the two probe tones). From Eq. (S4), the Hamiltonian Eq. (S16) is specified in an interaction picture defined by the Hamiltonian

$$\hat{H}_0 = (\omega_{\rm c} + \Omega + \bar{\delta})\hat{a}^\dagger\hat{a} + (\omega_{\rm d} + \bar{\delta}_{\rm d})\hat{a}^\dagger_{\rm d}\hat{a}_{\rm d} + (\bar{\omega} + \Delta)\left(\hat{b}^\dagger_1\hat{b}_1 + \hat{b}^\dagger_2\hat{b}_2\right). \tag{S17}$$

Note that the ideal experimental scenario referred to above now corresponds to $\bar{\delta} = \Delta = 0$ and $\bar{\delta}_{\rm d} = -\Omega$.

It is useful to introduce effective cavity quadrature operators, defined by $\hat{X}_{\rm (d)} = \left(\hat{a}_{\rm (d)} + \hat{a}^\dagger_{\rm (d)}\right)/\sqrt{2}$ and $\hat{P}_{\rm (d)} = -i\left(\hat{a}_{\rm (d)} - \hat{a}^\dagger_{\rm (d)}\right)/\sqrt{2}$, and collective mechanical quadrature operators, $\hat{X}_\pm = (\hat{X}_2 \pm \hat{X}_1)/\sqrt{2}$ and $\hat{P}_\pm = (\hat{P}_2 \pm \hat{P}_1)/\sqrt{2}$, where $\hat{X}_j = (\hat{b}_j + \hat{b}^\dagger_j)/\sqrt{2}$ and $\hat{P}_j = -i(\hat{b}_j - \hat{b}^\dagger_j)/\sqrt{2}$ for $j = 1, 2$ are the individual mechanical oscillator quadrature operators. The Hamiltonian Eq. (S16) can then be written in terms of these quadrature operators as

$$\begin{aligned}\hat{H} = &-\frac{\Omega+\bar{\delta}}{2}(\hat{X}^2 + \hat{P}^2) - \frac{\Omega+\bar{\delta}_{\rm d}}{2}(\hat{X}^2_{\rm d} + \hat{P}^2_{\rm d}) + \Omega(\hat{X}_+\hat{X}_- + \hat{P}_+\hat{P}_-) + \frac{\Delta}{2}\left(\hat{X}^2_+ + \hat{P}^2_+ + \hat{X}^2_- + \hat{P}^2_-\right)\\ &+\sqrt{2}(G_-\cos\psi_- + G_+\cos\psi_+)\hat{X}_+\hat{X} + \sqrt{2}(G_-\cos\psi_- - G_+\cos\psi_+)\hat{P}_+\hat{P}\\ &+\sqrt{2}(G_-\sin\psi_- + G_+\sin\psi_+)\hat{X}_+\hat{P} - \sqrt{2}(G_-\sin\psi_- - G_+\sin\psi_+)\hat{P}_+\hat{X}\\ &+\sqrt{2}(G^{\rm m}_-\cos\psi_- + G^{\rm m}_+\cos\psi_+)\hat{X}_-\hat{X} + \sqrt{2}(G^{\rm m}_-\cos\psi_- - G^{\rm m}_+\cos\psi_+)\hat{P}_-\hat{P}\\ &+\sqrt{2}(G^{\rm m}_-\sin\psi_- + G^{\rm m}_+\sin\psi_+)\hat{X}_-\hat{P} - \sqrt{2}(G^{\rm m}_-\sin\psi_- - G^{\rm m}_+\sin\psi_+)\hat{P}_-\hat{X}\\ &+\sqrt{2}(g_- + g_+)(\cos\phi\hat{X}_+ + \sin\phi\hat{P}_+)\hat{X}_{\rm d} + \sqrt{2}(g^{\rm m}_- + g^{\rm m}_+)(\cos\phi\hat{X}_- + \sin\phi\hat{P}_-)\hat{X}_{\rm d}\\ &+\sqrt{2}(g_- - g_+)(\cos\phi\hat{P}_+ - \sin\phi\hat{X}_+)\hat{P}_{\rm d} + \sqrt{2}(g^{\rm m}_- - g^{\rm m}_+)(\cos\phi\hat{P}_- - \sin\phi\hat{X}_-)\hat{P}_{\rm d},\end{aligned} \tag{S18}$$

where the effective optomechanical coupling rates are given by

$$G_\pm = (g_1 + g_2)\alpha_\pm/2, \qquad g_\pm = (g_1 + g_2)\alpha^{\rm d}_\pm/2, \tag{S19a}$$

$$G^{\rm m}_\pm = (g_1 - g_2)\alpha_\pm/2, \qquad g^{\rm m}_\pm = (g_1 - g_2)\alpha^{\rm d}_\pm/2, \tag{S19b}$$

with the m superscript denoting terms arising due to the mismatch in the single-photon optomechanical coupling rates, $g_1$ and $g_2$.

According to the Hamiltonian Eq. (S18), the probe tones (assuming they are set at the back-action evasion condition, $\alpha^{\rm d}_+ = \alpha^{\rm d}_-$) measures the collective mechanical quadrature,

$$X^{\rm d}_+ = \cos\phi X_+ + \sin\phi P_+\,, \tag{S20}$$

which has itself been defined in terms of a set of *rotated* mechanical collective quadratures, defined by

$$X_\pm = \cos\theta\hat{X}_\pm \pm \sin\theta\hat{X}_\mp\,, \tag{S21a}$$

$$P_\pm = \cos\theta\hat{P}_\pm \pm \sin\theta\hat{P}_\mp\,, \tag{S21b}$$

where the rotation angle is defined in terms of the single-photon optomechanical coupling rates via

$$\tan\theta = \frac{g_1 - g_2}{g_1 + g_2}. \tag{S22}$$

For the purpose of calculating noise spectra, it is convenient to rewrite the Hamiltonian Eq. (S18) in terms of the

rotated quadratures Eq. (S21a) and Eq. (S21b),

$$\begin{aligned}
\hat{H} =& -\frac{\Omega+\bar{\delta}}{2}(\hat{X}^2+\hat{P}^2) - \frac{\Omega+\bar{\delta}_{\mathrm{d}}}{2}(\hat{X}_{\mathrm{d}}^2+\hat{P}_{\mathrm{d}}^2) + \Omega_{\mathrm{c}}(X_+X_- + P_+P_-) + \frac{\Omega_{\mathrm{s}}}{2}(X_+^2+P_+^2-X_-^2-P_-^2) \\
&+\frac{\Delta}{2}\left(X_+^2+P_+^2+X_-^2+P_-^2\right) + \sqrt{2}\bar{g}_+X_+^{\mathrm{d}}\hat{X}_{\mathrm{d}} + \sqrt{2}\bar{g}_-\mathrm{sgn}(g_- - g_+)P_+^{\mathrm{d}}\hat{P}_{\mathrm{d}} \\
&+\sqrt{2}\frac{1}{\bar{G}_+}\left[\left(\cos\psi_- G_{-+}^2 + \cos\psi_+ G_{++}^2\right)X_+ - \left(\cos\psi_- - \cos\psi_+\right)G_\times^2 X_-\right]\hat{X} \\
&+\sqrt{2}\frac{1}{\bar{G}_-}\mathrm{sgn}(G_- - G_+)\left[\left(\cos\psi_- G_{--}^2 - \cos\psi_+ G_{+-}^2\right)P_+ + \left(\cos\psi_- - \cos\psi_+\right)G_\times^2 P_-\right]\hat{P} \\
&+\sqrt{2}\frac{1}{\bar{G}_+}\left[\left(\sin\psi_- G_{-+}^2 + \sin\psi_+ G_{++}^2\right)X_+ - \left(\sin\psi_- - \sin\psi_+\right)G_\times^2 X_-\right]\hat{P} \\
&+\sqrt{2}\frac{1}{\bar{G}_-}\mathrm{sgn}(G_- - G_+)\left[-\left(\sin\psi_- G_{--}^2 - \sin\psi_+ G_{+-}^2\right)P_+ - \left(\sin\psi_- - \sin\psi_+\right)G_\times^2 P_-\right]\hat{X},
\end{aligned} \tag{S23}$$

where $P_+^{\mathrm{d}} = \cos\phi P_+ - \sin\phi X_+$ is the observable canonically conjugate to $X_+^{\mathrm{d}}$ introduced in Eq. (S20), the effective optomechanical coupling rates are now given by

$$\bar{g}_\pm = \sqrt{(g_- \pm g_+)^2 + (g_-^{\mathrm{m}} \pm g_+^{\mathrm{m}})^2} = \sqrt{\frac{g_1^2+g_2^2}{2}(\alpha_-^{\mathrm{d}} \pm \alpha_+^{\mathrm{d}})^2}, \tag{S24a}$$

$$\bar{G}_\pm = \sqrt{(G_- \pm G_+)^2 + (G_-^{\mathrm{m}} \pm G_+^{\mathrm{m}})^2} = \sqrt{\frac{g_1^2+g_2^2}{2}(\alpha_- \pm \alpha_+)^2}, \tag{S24b}$$

$$G_\times^2 = G_-G_+^{\mathrm{m}} - G_+G_-^{\mathrm{m}}, \tag{S24c}$$

$$G_{-\pm}^2 = G_-(G_- \pm G_+) + G_-^{\mathrm{m}}(G_-^{\mathrm{m}} \pm G_+^{\mathrm{m}}), \tag{S24d}$$

$$G_{+\pm}^2 = G_+(G_- \pm G_+) + G_+^{\mathrm{m}}(G_-^{\mathrm{m}} \pm G_+^{\mathrm{m}}), \tag{S24e}$$

and the asymmetry in the optomechanical couplings is parametrised as

$$\Omega_{\mathrm{c}} = \Omega\cos 2\theta, \qquad \Omega_{\mathrm{s}} = \Omega\sin 2\theta. \tag{S25}$$

Now recall that quantum entanglement between two oscillators (mechanical oscillators 1 and 2 here) may be indicated by the Duan inequality [7]. In terms of the original mechanical collective quadrature operators this is $\langle\hat{X}_+^2\rangle + \langle\hat{P}_-^2\rangle < 1$. In terms of the rotated mechanical collective quadrature operators, Eq. (S21a) and Eq. (S21b), the Duan inequality takes the form [8]

$$\langle X_+^2\rangle + \langle P_-^2\rangle < \cos 2\theta. \tag{S26}$$

In the experiment $g_1/g_2 = 0.98$, and the right-hand side of Eq. (S26) is 0.9998; i.e., 1 for all practical purposes.

### C. Heisenberg-Langevin equations

The dynamics corresponding to the Hamiltonian Eq. (S23) and damping of the oscillator modes into independent thermal baths is readily described by a system of linear Heisenberg-Langevin equations [10],

$$\frac{d}{dt}\vec{Z} = \mathbf{A}\cdot\vec{Z} + \mathbf{B}\cdot\vec{Z}^{\mathrm{in}}. \tag{S27}$$

Here $\vec{Z} = (X_+, P_-, X_-, P_+, X, P, X_{\mathrm{d}}, P_{\mathrm{d}})^T$ is a vector of rotated collective mechanical quadrature operators and cavity quadrature operators, $\vec{Z}^{\mathrm{in}} = \left(X_+^{\mathrm{in}}, P_-^{\mathrm{in}}, X_-^{\mathrm{in}}, P_+^{\mathrm{in}}, X_{\mathrm{E}}^{\mathrm{in}}, P_{\mathrm{E}}^{\mathrm{in}}, X_{\mathrm{pE}}^{\mathrm{in}}, P_{\mathrm{pE}}^{\mathrm{in}}, X_{\mathrm{I}}^{\mathrm{in}}, P_{\mathrm{I}}^{\mathrm{in}}, X_{\mathrm{pI}}^{\mathrm{in}}, P_{\mathrm{pI}}^{\mathrm{in}}\right)^T$ is the vector of corresponding delta-correlated quadrature input noise operators, $\mathbf{A}$ is an eight-by-eight constant matrix, and $\mathbf{B}$ is an eight-by-twelve constant matrix. Note that the cavity mode input noise arises from both external (subscript E) and internal (subscript I) cavity damping. The symmetrically-ordered, steady-state covariance matrix for the quadrature operators, $\mathbf{V}$, follows from solution of the Lyapunov equation corresponding to Eq. (S27),

$$\mathbf{AV} + \mathbf{VA}^{\mathrm{T}} + \mathbf{BB}^{\mathrm{T}} = \mathbf{0}. \tag{S28}$$

Now the matrix $\mathbf{A}$ may be specified via a four-by-four array of two-by-two block matrices, $\mathbf{A}_{ij}$ ($j = 1,2,3,4$). Assuming that $G_- \geq G_+$ and $g_- \geq g_+$ in Eq. (S23), the non-zero $\mathbf{A}_{ij}$ are

$$\mathbf{A}_{11} = \mathbf{A}_{22} = \begin{bmatrix} -\bar{\gamma}/2 & \Omega_\mathrm{c} \\ -\Omega_\mathrm{c} & -\bar{\gamma}/2 \end{bmatrix}, \tag{S29a}$$

$$\mathbf{A}_{33} = \begin{bmatrix} -\kappa/2 & -(\Omega + \bar{\delta}) \\ \Omega + \bar{\delta} & -\kappa/2 \end{bmatrix}, \quad \mathbf{A}_{44} = \begin{bmatrix} -\kappa/2 & -(\Omega + \bar{\delta}_\mathrm{d}) \\ \Omega + \bar{\delta}_\mathrm{d} & -\kappa/2 \end{bmatrix}, \tag{S29b}$$

$$\mathbf{A}_{12} = \begin{bmatrix} -\gamma_\mathrm{m}/2 & \Omega_\mathrm{s} + \Delta \\ \Omega_\mathrm{s} - \Delta & -\gamma_\mathrm{m}/2 \end{bmatrix}, \quad \mathbf{A}_{21} = \begin{bmatrix} -\gamma_\mathrm{m}/2 & -\Omega_\mathrm{s} + \Delta \\ -\Omega_\mathrm{s} - \Delta & -\gamma_\mathrm{m}/2 \end{bmatrix}, \tag{S29c}$$

$$\mathbf{A}_{14} = \begin{bmatrix} \sqrt{2}\bar{g}_+ \sin\phi & \sqrt{2}\bar{g}_- \cos\phi \\ 0 & 0 \end{bmatrix}, \quad \mathbf{A}_{24} = \begin{bmatrix} 0 & 0 \\ -\sqrt{2}\bar{g}_+ \cos\phi & \sqrt{2}\bar{g}_- \sin\phi \end{bmatrix}, \tag{S29d}$$

$$\mathbf{A}_{41} = \begin{bmatrix} -\sqrt{2}\bar{g}_- \sin\phi & 0 \\ -\sqrt{2}\bar{g}_+ \cos\phi & 0 \end{bmatrix}, \quad \mathbf{A}_{42} = \begin{bmatrix} 0 & \sqrt{2}\bar{g}_- \cos\phi \\ 0 & -\sqrt{2}\bar{g}_+ \sin\phi \end{bmatrix}, \tag{S29e}$$

$$\mathbf{A}_{13} = \sqrt{2} \begin{bmatrix} (\sin\psi_- G_{--}^2 - \sin\psi_+ G_{+-}^2)/\bar{G}_- & (\cos\psi_- G_{--}^2 - \cos\psi_+ G_{+-}^2)/\bar{G}_- \\ (\cos\psi_- - \cos\psi_+) G_\times^2/\bar{G}_+ & (\sin\psi_- - \sin\psi_+) G_\times^2/\bar{G}_+ \end{bmatrix}, \tag{S29f}$$

$$\mathbf{A}_{23} = \sqrt{2} \begin{bmatrix} -(\sin\psi_- - \sin\psi_+) G_\times^2/\bar{G}_- & (\cos\psi_- - \cos\psi_+) G_\times^2/\bar{G}_- \\ -(\cos\psi_- G_{-+}^2 + \cos\psi_+ G_{++}^2)/\bar{G}_+ & -(\sin\psi_- G_{-+}^2 + \sin\psi_+ G_{++}^2)/\bar{G}_+ \end{bmatrix}, \tag{S29g}$$

$$\mathbf{A}_{31} = \sqrt{2} \begin{bmatrix} (\sin\psi_- G_{-+}^2 + \sin\psi_+ G_{++}^2)/\bar{G}_+ & (\cos\psi_- - \cos\psi_+) G_\times^2/\bar{G}_- \\ -(\cos\psi_- G_{-+}^2 + \cos\psi_+ G_{++}^2)/\bar{G}_+ & (\sin\psi_- - \sin\psi_+) G_\times^2/\bar{G}_- \end{bmatrix}, \tag{S29h}$$

$$\mathbf{A}_{32} = \sqrt{2} \begin{bmatrix} -(\sin\psi_- - \sin\psi_+) G_\times^2/\bar{G}_+ & (\cos\psi_- G_{--}^2 - \cos\psi_+ G_{+-}^2)/\bar{G}_- \\ (\cos\psi_- - \cos\psi_+) G_\times^2/\bar{G}_+ & (\sin\psi_- G_{--}^2 - \sin\psi_+ G_{+-}^2)/\bar{G}_- \end{bmatrix}, \tag{S29i}$$

where the average and half-difference mechanical damping rates have been introduced as

$$\bar{\gamma} = \frac{\gamma_1 + \gamma_2}{2}, \tag{S30a}$$

$$\gamma_\mathrm{m} = \frac{\gamma_1 - \gamma_2}{2}, \tag{S30b}$$

respectively. The matrix $\mathbf{B}$ may be specified via a four-by-six array of two-by-two block matrices, $\mathbf{B}_{ij}$ ($i, j = 1, 2, \ldots, 6$). The non-zero $\mathbf{B}_{ij}$ are

$$\mathbf{B}_{11} = \mathbf{B}_{22} = \sqrt{\gamma_+}\mathbf{I}_2, \quad \mathbf{B}_{12} = \mathbf{B}_{21} = \sqrt{\gamma_-}\mathbf{I}_2, \tag{S31a}$$

$$\mathbf{B}_{33} = \mathbf{B}_{44} = \sqrt{\kappa_\mathrm{E}(n_\mathrm{E}^\mathrm{T} + 1/2)}\,\mathbf{I}_2, \tag{S31b}$$

$$\mathbf{B}_{35} = \mathbf{B}_{46} = \sqrt{\kappa_\mathrm{I}(n_\mathrm{I}^\mathrm{T} + 1/2)}\,\mathbf{I}_2, \tag{S31c}$$

$$2\sqrt{\gamma_\pm} = \sqrt{\gamma_1(n_1^\mathrm{T} + 1/2)} \pm \sqrt{\gamma_2(n_2^\mathrm{T} + 1/2)}, \tag{S31d}$$

where $n_\mathrm{E}^\mathrm{T}$ and $n_\mathrm{I}^\mathrm{T}$ denote effective thermal occupations of external and internal cavity baths, and $n_1^\mathrm{T}$ and $n_2^\mathrm{T}$ denote effective thermal occupations of the baths for mechanical oscillators 1 and 2, respectively. We usually work in terms of the actual cavity temperature given by

$$n_\mathrm{c}^\mathrm{T} = \frac{n_\mathrm{I}^\mathrm{T}\kappa_\mathrm{I} + n_\mathrm{E}^\mathrm{T}\kappa_\mathrm{E}}{\kappa}. \tag{S32}$$

### D. Noise spectra

The directly measurable quantity in this experiment is the cavity noise spectrum, which may then be used to infer the noise spectra of the collective mechanical quadratures. Contributions to the cavity spectrum will arise from the thermal fluctuations of the cavity, and from both the pump and probe tones. The normally-ordered cavity noise spectrum may be calculated in terms of normally-ordered spectral contributions as

$$S[\omega] = S_\mathrm{d}[\omega] + \bar{S}[\omega] - S_\mathrm{d}^\mathrm{u}[\omega], \tag{S33}$$

where $S_{\rm d}[\omega]$ is the spectral contribution due to the probe tones,

$$S_{\rm d}[\omega] = \lim_{t\to\infty} 2\,{\rm Re}\int_0^{+\infty} d\tau\, e^{-i\omega\tau}\langle \hat{a}_{\rm d}^\dagger(t+\tau)\hat{a}_{\rm d}(t)\rangle, \tag{S34}$$

$\bar{S}[\omega]$ is the spectral contribution due to the pump tones (expressed in the reference frame of the probe tones),

$$\bar{S}[\omega] = \lim_{t\to\infty} 2\,{\rm Re}\int_0^{+\infty} d\tau\, e^{-i\omega\tau}e^{-i(\bar{\delta}-\bar{\delta}_{\rm d})\tau}\langle \hat{a}(t+\tau)\hat{a}(t)\rangle, \tag{S35}$$

and $S_{\rm d}^{\rm u}[\omega] \equiv S_{\rm d}[\omega]|_{\bar{g}_\pm=0}$ is the noise spectrum of the cavity mode uncoupled from the mechanical modes. The latter quantity must be subtracted in Eq. (S33) so that the thermal fluctuations of the cavity mode are not counted twice.

Using $\hat{a}_{(\rm d)}(t) = \left(\hat{X}_{(\rm d)}(t) + i\hat{P}_{(\rm d)}(t)\right)/\sqrt{2}$, the correlation functions in Eqs. (S34) and Eq. (S35) are readily expanded in terms of quadrature correlation functions. We now briefly describe the evaluation of these quadrature correlation functions. Taking quantum expectations of Eq. (S27) and writing the result in component form we get

$$\frac{d}{dt}\langle Z_i(t)\rangle = \sum_{j=1}^{8} a_{ij}\langle Z_j(t)\rangle, \tag{S36}$$

for $i = 1, 2, \ldots, 8$, where $a_{ij}$ denotes the $(i,j)^{\rm th}$ component of the matrix $\mathbf{A}$, and $Z_i(t)$ denotes the $i^{\rm th}$ component of the vector $\vec{Z}(t)$. The quantum regression theorem [9] then tells us that the corresponding correlation functions obey

$$\frac{\partial}{\partial\tau}\langle Z_i(t+\tau)Z_k(t)\rangle = \sum_{j=1}^{8} a_{ij}\langle Z_j(t+\tau)Z_k(t)\rangle, \tag{S37}$$

for $i, k = 1, 2, \ldots, 8$. Now one can construct an $8\times 8$ matrix of correlation functions $\langle Z_i(t+\tau)Z_k(t)\rangle$, and then convert it into a 64-dimensional row-major vector, which we denote by $\vec{V}(t,\tau)$. From Eq. (S37), we find that $\vec{V}(t,\tau)$ obeys

$$\frac{\partial}{\partial\tau}\vec{V}(t,\tau) = \mathbf{C}\,\vec{V}(t,\tau), \tag{S38}$$

where $\mathbf{C}$ is a $64\times 64$ matrix with elements given by $c_{8(i-1)+k,8(j-1)+k} = a_{ij}$ for $i, j, k = 1, 2, \ldots, 8$. Eq. (S38) is readily solved by diagonalisation, and the steady-state correlation functions follow as

$$\lim_{t\to\infty}\vec{V}(t,\tau) = \mathbf{D}\,e^{\mathbf{D}^{-1}\mathbf{C}\mathbf{D}\tau}\,\mathbf{D}^{-1}\lim_{t\to\infty}\vec{V}(t,0), \tag{S39}$$

where $\mathbf{D}$ is the matrix of eigenvectors of $\mathbf{C}$ and $\lim_{t\to\infty}\vec{V}(t,0)$ is the row-major vector corresponding to the unsymmetrized form of $\mathbf{V}$. The quadrature autocorrelation functions of interest may be extracted as elements of the vector in Eq. (S39),

$$\lim_{t\to\infty}\langle Z_i(t+\tau)Z_i(t)\rangle = \lim_{t\to\infty}\left[\vec{V}(t,\tau)\right]_{9(i-1)+1}, \tag{S40}$$

for $i = 1, 2, \ldots, 8$.

The contribution to the overall spectrum Eq. (S33) associated with the probe tones is readily obtained numerically using Eqs. (S28), (S34), (S39) and (S40). The contribution to the overall spectrum Eq. (S33) associated with the pump tones (in the reference frame of the probe tones) is readily obtained numerically using Eqs. (S28), (S35), (S39), and (S40).

At this point we quote some analytical results, although we stress all the results are verified using the full numerical model. The probe tone spectrum may be obtained analytically under mild assumptions, in terms of the mechanical noise spectra. We may consider the Hamiltonian Eq. (S23) under the assumption $\bar{G}_\pm \gg \bar{g}_\pm$; that is, the pump tones are much stronger than the probe tones. Then the dynamics, steady-state, and fluctuations of the mechanical oscillators, will be largely unaffected by their couplings to the cavity mode via the probe tones. Hence, we may calculate $S_{X_+}[\omega]$, defined by

$$S_{X_+}[\omega] = \lim_{t\to\infty} 2\,{\rm Re}\int_0^{+\infty} d\tau\, e^{-i\omega\tau}\langle X_+(t+\tau)X_+(t)\rangle, \tag{S41}$$

without reference to the probe tones, and then calculate the spectral contribution associated with the probe tones, $S_{\rm d}[\omega]$, independently of the pump tone contribution under the assumption that $\left|\bar{\delta}-\bar{\delta}_{\rm d}\right| \gg \bar{\gamma}$. Under the assumption of back-action evading probe tones ($\alpha_{-}^{\rm d}=\alpha_{+}^{\rm d}$) and $\phi=0$, we find the noise spectrum

$$S_{\rm d}[\omega]=\frac{4\bar{g}_{+}^{2}}{\kappa^{2}+4(\omega+\Omega+\bar{\delta}_{\rm d})^{2}}S_{X_{+}}[\omega]+\frac{4\kappa_{\rm I}}{\kappa^{2}+4(\omega+\Omega+\bar{\delta}_{\rm d})^{2}}n_{\rm I}^{\rm T}+\frac{4\kappa_{\rm E}}{\kappa^{2}+4(\omega+\Omega+\bar{\delta}_{\rm d})^{2}}n_{\rm E}^{\rm T}. \tag{S42}$$

In the absence of any coupling to the mechanical modes ($\bar{g}_{\pm}=0$), this spectral contribution becomes

$$S_{\rm d}^{\rm u}[\omega]=\frac{4(\kappa_{\rm I}n_{\rm I}^{\rm T}+\kappa_{\rm E}n_{\rm E}^{\rm T})}{\kappa^{2}+4(\omega+\Omega+\bar{\delta}_{\rm d})^{2}}. \tag{S43}$$

Finally, the normally-ordered cavity output spectrum follows from the normally-ordered cavity spectrum as [10, 11]

$$S_{\rm out}[\omega]=\lim_{t\to\infty}2\,{\rm Re}\int_{0}^{+\infty}d\tau\,e^{-i\omega\tau}\langle\hat{a}_{\rm out}^{\dagger}(t+\tau)\hat{a}_{\rm out}(t)\rangle=\kappa_{\rm E}S[\omega], \tag{S44}$$

where $S[\omega]$ is the spectrum defined in Eq. (S33).

In any case, including the general numerical evaluation of the quantities, the variance of the $X_{+}$ quadrature is calculated from the corresponding spectral density $S_{X_{+}}[\omega]$ in Eq. (S41) as

$$\langle X_{+}^{2}\rangle=\frac{1}{2\pi}\int d\omega S_{X_{+}}[\omega]\,, \tag{S45}$$

and similarly for other collective mechanical quadratures.

## II. EXPERIMENTAL CALIBRATIONS

### A. Probe spectrum

We now discuss calibration of the probe spectrum that starts by using thermal states of the mechanical oscillators. We describe the analytical model that we also have verified using full numerics for the current set of parameters including all asymmetries. The mechanical contribution to the probe output spectrum is given by Eqs. (S42,S44) as

$$S_{\rm out}^{\rm d}[\omega]=\frac{4\bar{g}_{+}^{2}\kappa_{\rm E}}{\kappa^{2}+4(\omega+\Omega+\bar{\delta}_{\rm d})^{2}}S_{X_{+}}[\omega]\,. \tag{S46}$$

The output photon flux follows as the integrated output spectrum

$$n_{\rm out}^{\rm d}\equiv\frac{1}{2\pi}\int_{-\infty}^{+\infty}d\omega\,S_{\rm out}^{\rm d}[\omega]=\frac{4\bar{g}_{+}^{2}\kappa_{\rm E}}{\kappa^{2}+4(\omega+\Omega+\bar{\delta}_{\rm d})^{2}}\langle X_{+}^{2}\rangle\,. \tag{S47}$$

#### 1. *Thermal state of the mechanics*

In order to write down the spectrum of a thermal state of the two-oscillator system, we define a sum of two Lorentzians:

$$S_{0}[\omega]=\frac{\gamma/2}{\gamma^{2}/4+(\omega-\Omega)^{2}}+\frac{\gamma/2}{\gamma^{2}/4+(\omega+\Omega)^{2}}\,. \tag{S48}$$

Then it holds that

$$S_{\rm X_{+}}[\omega]=\frac{1}{2}(1+n_{1}^{\rm T}+n_{2}^{\rm T})S_{0}[\omega], \tag{S49}$$

In thermal state, the variance and the flux are, based on Eqs. (S45,S49)

$$\langle X_{+}^{2}\rangle^{\rm T}=\frac{1}{2}\left(n_{1}^{\rm T}+n_{2}^{\rm T}+1\right)\,, \tag{S50}$$

$$n_{\rm out}^{\rm T}=\frac{4\bar{g}_{+}^{2}\kappa_{\rm E}}{\kappa^{2}+4(\omega+\Omega+\bar{\delta}_{\rm d})^{2}}\langle X_{+}^{2}\rangle^{\rm T}=\frac{2\bar{g}_{+}^{2}\kappa_{\rm E}}{\kappa^{2}+4(\omega+\Omega+\bar{\delta}_{\rm d})^{2}}\left(n_{1}^{\rm T}+n_{2}^{\rm T}+1\right)\,. \tag{S51}$$

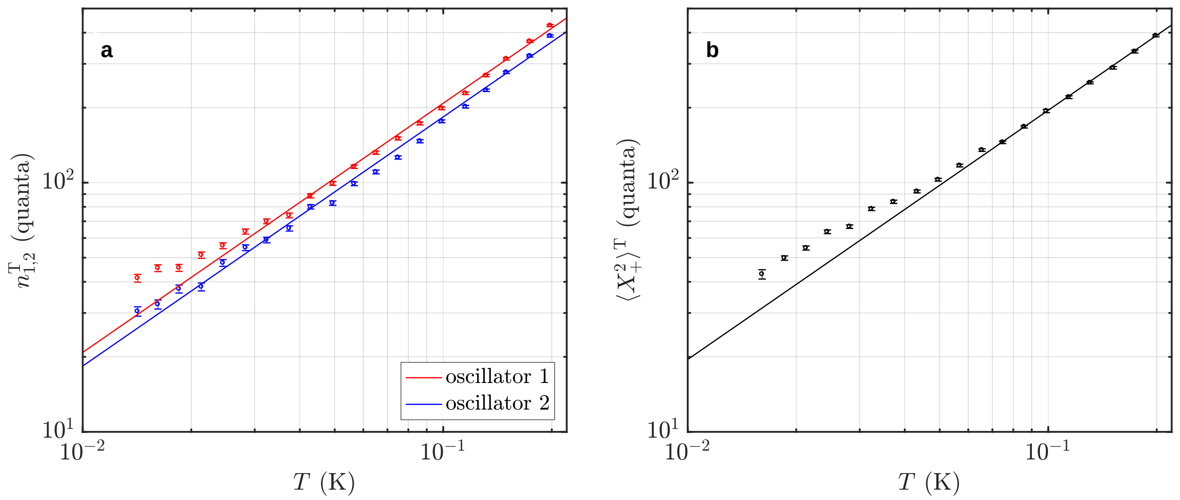


FIG. S1. *Thermal calibrations.* **a**, A single weak red tone. **b**, Two-mode BAE conditions. The solid lines are linear fits.

The measured quantity $S_{\mathrm{o}}^{\mathrm{d}}[\omega]$ is the output field Eq. (S46) right after the sample, multiplied by the total gain $\mathcal{A}$ of the detection chain:

$$S_{\mathrm{o}}^{\mathrm{d}}[\omega] = \mathcal{A} S_{\mathrm{out}}^{\mathrm{d}}[\omega] \ + \text{noise floor}\,. \tag{S52}$$

The field amplitude squared is proportional to the generator power setting $P_{\mathrm{d}}$ through a chain of unknown attenuation stages, and of the cavity driving, which we incorporate into a proportionality constant $\mathcal{M}$, such that the probe effective coupling is written as

$$\bar{g}_+^2 = \mathcal{M} P_{\mathrm{d}}\,. \tag{S53}$$

From the measured spectrum Eq. (S52), we reconstruct the mechanical spectrum using Eqs. (S46,S53):

$$S_{X_+}[\omega] = \frac{S_{\mathrm{o}}^{\mathrm{d}}[\omega]}{\mathcal{A}\mathcal{M}} \frac{\kappa^2 + 4(\omega + \Omega + \bar{\delta}_{\mathrm{d}})^2}{4 P_{\mathrm{d}} \kappa_{\mathrm{E}}}\,. \tag{S54}$$

Similarly, the integrated quantity

$$n_{\mathrm{o}}^{\mathrm{d}} = \mathcal{A} n_{\mathrm{out}}^{\mathrm{d}} = \frac{1}{2\pi} \int_{-\infty}^{+\infty} d\omega \, S_{\mathrm{o}}^{\mathrm{d}}[\omega] \tag{S55}$$

gives the variance of a quadrature according to Eq. (S47):

$$\langle X_+^2 \rangle = \frac{n_{\mathrm{o}}^{\mathrm{d}}}{\mathcal{A}\mathcal{M}} \frac{\kappa^2 + 4(\omega + \Omega + \bar{\delta}_{\mathrm{d}})^2}{4 P_{\mathrm{d}} \kappa_{\mathrm{E}}}\,. \tag{S56}$$

In order to use Eq. (S54), Eq. (S56), we need to calibrate the quantity $\mathcal{A}\mathcal{M}$ that involves the gain, as well as the effective probe coupling at a given generator power. The gain includes the gains of the amplifiers as well as losses in the cables following the sample.

### B. Thermal calibrations

It is well established that under pumping with a single weak tone, a linear temperature dependence of the sideband peak area serves as an accurate calibration of the mechanical mode temperature. In Fig. S1a we display such an experiment, indicating that there is some decoupling from the cryostat bath below 30 mK in particular for oscillator 1.

In the thermal calibration of the two-mode BAE signal, we use a small coupling $\bar{g}_+ = \bar{g}_{+,0}$ that does not heat up the system. Lorentzians are fitted to the two peaks in the measured probe output spectrum. The sum area of the two peaks from Eq. (S51) is

$$n_\mathrm{o}^\mathrm{T} = \mathcal{A} n_\mathrm{out}^\mathrm{T} = \mathcal{T}\langle X_+^2\rangle^\mathrm{T} = \mathcal{T}\left(\frac{k_B}{\hbar\omega_1} + \frac{k_B}{\hbar\omega_2}\right)T\,, \qquad \text{with} \quad \mathcal{T} = \mathcal{A}\frac{2\bar{g}_{+,0}^2\kappa_\mathrm{E}}{\kappa^2 + 4(\omega+\Omega+\bar{\delta}_\mathrm{d})^2}\,. \tag{S57}$$

We fit a straight line to the measured $n_\mathrm{o}^\mathrm{T}$, allowing us to find

$$\langle X_+^2\rangle^\mathrm{T} = \frac{n_\mathrm{o}^\mathrm{T}}{\mathcal{T}}\,. \tag{S58}$$

In particular, we find in the analysis presented in Fig. S1b that the minimum thermal occupation at $T \simeq 15$ mK is $\langle X_+^2\rangle_0 \simeq 41$.

### C. Power calibration of BAE signal

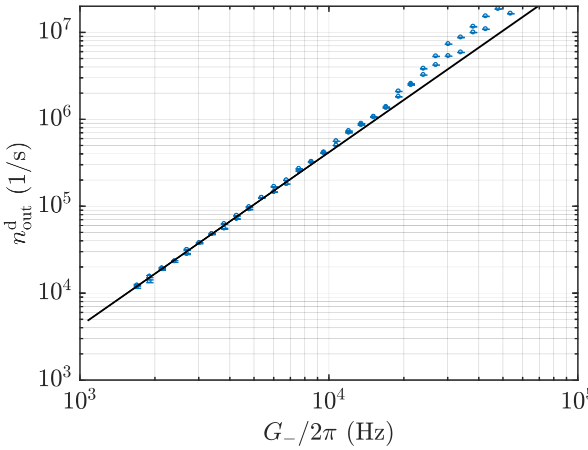


FIG. S2. *Probe power calibration.* The solid line is a fit according to Eq. (S59).

The probe powers we use in the two-mode squeezing detection are generally different and higher than those used in the thermal calibrations, so it is important to carefully calibrate the expected probe signal at a given probe power. We now use Eq. (S51) at the known occupation $\langle X_+^2\rangle^\mathrm{T} = \langle X_+^2\rangle_0$, but crank up the powers of the probe signal generators that affects the probe coupling $\bar{g}_+$, while keeping the power ratio fixed in order to retain the BAE conditions. We fit a straight line to the peak area as a function of generator power (we select $P_\mathrm{d}$ to denote the red-detuned probe generator power setting), obtaining the calibration coefficient $\mathcal{N}$:

$$n_\mathrm{o}^\mathrm{d} = \mathcal{A} n_\mathrm{out}^\mathrm{d} = \mathcal{N} P_\mathrm{d}\,. \tag{S59}$$

Combining with Eq. (S51) we obtain

$$\mathcal{A}\mathcal{M} = \frac{\kappa^2 + 4(\omega+\Omega+\bar{\delta}_\mathrm{d})^2}{4\kappa_\mathrm{E}\langle X_+^2\rangle_0}\mathcal{N}\,. \tag{S60}$$

We insert Eq. (S60) into Eq. (S54) and Eq. (S56), finally obtaining the quadrature spectra and variance in terms of only calibrated quantities:

$$S_{X_+}[\omega] = \frac{S_\mathrm{o}[\omega]}{4P_\mathrm{d}}\frac{\kappa^2 + 4(\omega+\Omega+\bar{\delta}_\mathrm{d})^2}{\mathcal{A}\mathcal{M}\kappa_\mathrm{E}} = \frac{S_\mathrm{o}[\omega]}{P_\mathrm{d}}\frac{\langle X_+^2\rangle_0}{\mathcal{N}}\,, \tag{S61a}$$

$$\langle X_+^2\rangle = \frac{n_\mathrm{o}}{P_\mathrm{d}}\frac{\langle X_+^2\rangle_0}{\mathcal{N}}\,. \tag{S61b}$$

A value below $\langle X_+^2 \rangle = 1/2$ in Eq. (S61b) corresponds to two-mode squeezing below zero-point fluctuations. Equation (S61b) essentially tells that we calibrate the peak area at a given probe generator power and at a known phonon occupation, and this allows us to infer some other occupation at another generator power by simple scaling. Notice that although the details of the transduction of the signal, or of the system gain are present in the intermediate forms (e.g., $\kappa_{\rm E}$ in Eq. (S56)), these cancel in the end. One can then say that the approach is insensitive to detailed understanding of the system parameters or functioning.

The data for the probe power calibration (Eq. (S59)) is shown in Fig. S2. For convenience, the flux is here plotted in absolute units, obtained by dividing by the system gain $\mathcal{A}$ from sideband cooling calibration. Notice again that the calibration does not rely on knowing the absolute units. As seen in the figure, the area deviates from straight line at higher powers, consistent with heating of oscillator 1 (see Figs. S4, S5 below). The heating does not compromise the calibration, since the correct way of making linear fit at small powers, instead of trying to consider the points where heating affects, results in the most modest claim of entanglement.

### D. Effective couplings of the probes

The analysis in section II C, although allowing for precise measurement of the variance, does not allow for directly comparing the probe output spectrum to theory, because the absolute effective coupling $g_\pm$ at a given generator power is not accessable.

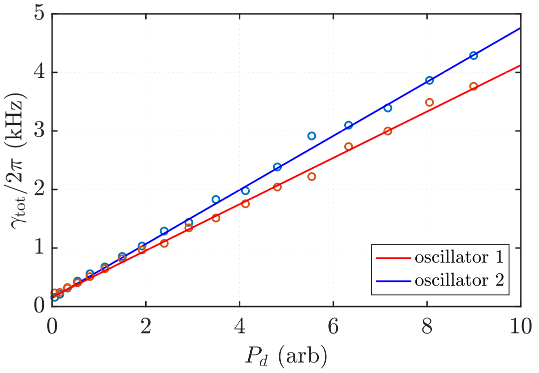


FIG. S3. *Effective couplings of the probes.* A single red-detuned probe tone was applied at the frequency $\omega_c - \Omega$.

In order to calibrate the latter, we apply a single red-detuned probe tone at the nominal middle-sideband frequency. At this point we have to separate the two oscillators by their slightly unequal single-photon couplings. The effective coupling for either individual oscillator $i = 1, 2$ is $g_{\rm i-} = g_{\rm i}\alpha_-^{\rm d}$, and we denote the calibration between generator power and coupling as $\mathcal{M}_{\rm i}$:

$$g_{\rm i-}^2 = \mathcal{M}_{\rm i} P_{\rm d} \,. \tag{S62}$$

The single red-detuned probe tone causes an enhanced damping of either mechanics by the amount

$$\gamma_{\rm opt,i} = \frac{4g_{\rm i-}^2\kappa}{\kappa^2 + 4(\Omega+\omega_{\rm i})^2} = \frac{4\mathcal{M}_{\rm i} P_{\rm d}\kappa}{\kappa^2 + 4(\Omega+\omega_{\rm i})^2} \,. \tag{S63}$$

We fit the damping as a function of signal generator power, obtaining

$$\gamma_{\rm opt,i} = \mathcal{H}_{\rm i} P_{\rm d} \,, \tag{S64}$$

and by combining Eq. (S63) and Eq. (S64) we find

$$\mathcal{M}_{\rm i} = \frac{\mathcal{H}_{\rm i}\left(\kappa^2 + 4(\Omega+\omega_{\rm i})^2\right)}{4\kappa} \,. \tag{S65}$$

Simultaneously we also obtain calibration of the ratio of the single-photon couplings of the two oscillators,

$$\frac{g_1}{g_2} = \frac{\mathcal{M}_1}{\mathcal{M}_2} \,, \tag{S66}$$

as shown in Fig. S3, with the result $g_1/g_2 \simeq 0.94 \pm 0.02$. In the final data fitting, we end up with $g_1/g_2 \simeq 0.98$ that is slightly off from the statistical error limits. This can be due to the fact that the probe tone was not applied exactly at the mid-sideband frequency. In principle we calibrated the said frequency based on the cavity linear response, but the latter is known to be slightly distorted by stray coupling.

### E. Effective couplings of the pumps

For the pumps, the effective coupling is calibrated in a similar manner to to the probe case. We apply a red-detuned pump tone, now at the red sideband of either mechanics. The calibration from the power $P_\mathrm{p}$ of the generator that provides the red pump tone, to the coupling is

$$G_{\mathrm{i}-}^2 = \mathcal{J}_\mathrm{i} P_\mathrm{p} \,, \tag{S67}$$

and the pump damping is

$$\gamma_{\mathrm{opt,i}} = \frac{4G_{\mathrm{i}-}^2}{\kappa} = \frac{4\mathcal{J}_\mathrm{i} P_\mathrm{p}}{\kappa} \,. \tag{S68}$$

We fit the damping as a function generator power, obtaining

$$\gamma_{\mathrm{opt,i}} = \mathcal{L}_\mathrm{i} P_\mathrm{p} \,, \tag{S69}$$

yielding the calibration coefficients in Eq. (S67)

$$\mathcal{J}_\mathrm{i} = \frac{\mathcal{L}_\mathrm{i}\kappa}{4} \,. \tag{S70}$$

The final effective coupling, including asymmetries, becomes

$$G_-^2 = \mathcal{J}_1/4 \left[1 + (g_2/g_1)\right]^2 P_\mathrm{p} \,. \tag{S71}$$

Having the pump effective couplings, we calibrate the system gain using the sideband cooling, which we selected as the calibration standard at this point because it offers a wide variety of different line profiles, and over a large dynamic range, to fit in. The measured pump output spectra $\bar{S}_\mathrm{o}[\omega]$ on top of the noise floor is

$$\bar{S}_\mathrm{o}[\omega] = \mathcal{A}\bar{S}_\mathrm{out}[\omega] \tag{S72}$$

are fitted using an analytical expression $\bar{S}_\mathrm{out}[\omega]$ that essentially is that in Ref. [12] applied for our cavity geometry.

We note that a similar approach does not allow an accurate calibration of what happens when the tone is applied at the blue sideband, because in the latter case the dynamic range is very limited by instability. We attempted to apply the calibration made for the red-detuned pump, however, this does not match the data. This indicates a frequency dependent attenuation in the system, as we observed with the blue-detuned probe as well. Hence, we calibrate the effective coupling $G_+$ using the cavity linear response, see Fig. S6.

At this point we mention that in all the modeling, we use a single-port cavity whereas in the experiment we have (asymmetric) double-sided cavity that hence has one more path where the total signal can split into. To this end we model the cavity as being effectively single-port with the output coupling equal to the true output coupling $\kappa_\mathrm{Eo}$, and the input port dissipation is included in an effective internal loss equal to $\kappa_\mathrm{I} + \kappa_\mathrm{Ei}$ that is used in place of an internal loss in the modeling.

### F. Additional data and list of parameters

In Fig. S7 we display the measured probe spectrum for dataset $D$ discussed in main text, having a higher pump power than dataset $C$. As mentioned, the peaks are somewhat shifted and rounded as compared to the theoretical expectation, a fact that we attribute to phase drift of the generators during data acquisition.

As mentioned above, the linear response of the cavity when the pump tones are on is a useful consistency check of the calibrations and fits. In Fig. S6 we display the $S_{21}$ transmission measurement pertaining to dataset $C$, together with a theoretical fit using the parameters fixed to that dataset. We note that the cavity transmission at microwave frequencies is easily distorted by stray transmission channels, and hence in particular the tails of the profile having the lowest transmission should not be taken as a foundation of a calibration.

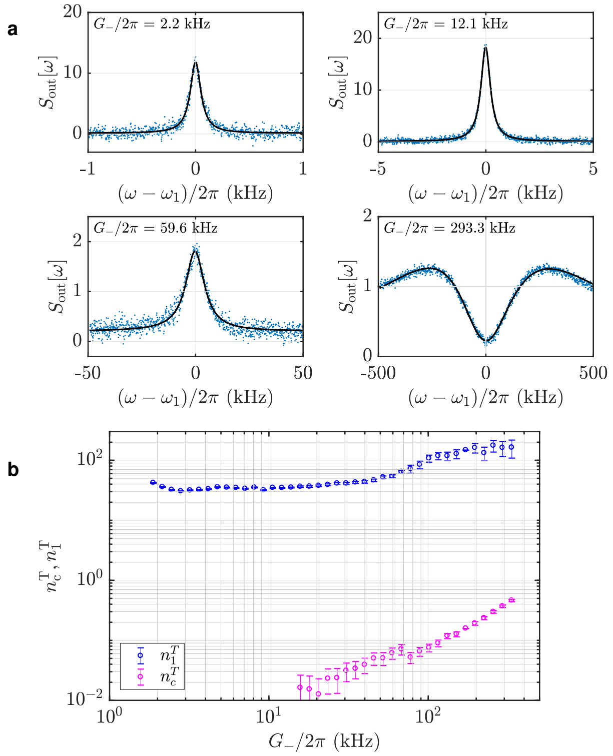


FIG. S4. *Sideband cooling, oscillator 1.* **a**, Spectra and theory fits at effective coupling values quoted in the panels. **b**, Extracted bath temperatures of oscillator 1 and of the cavity.

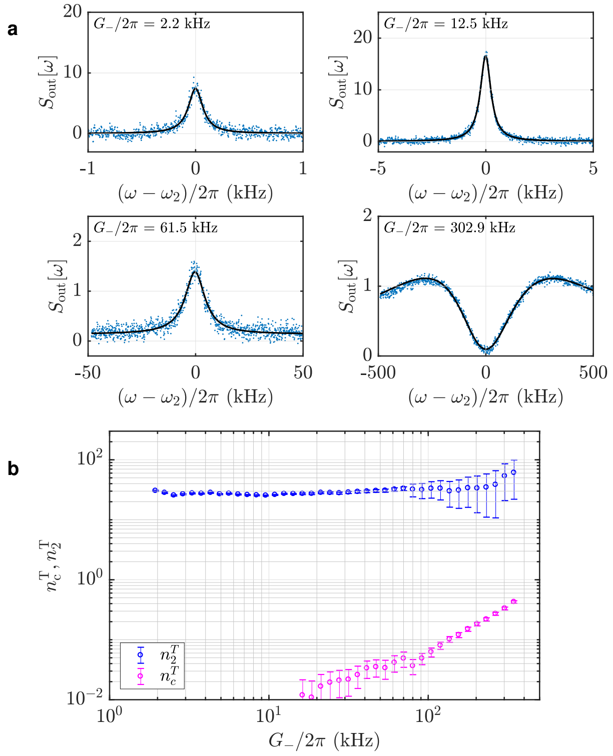


FIG. S5. *Sideband cooling, oscillator 2.* **a**, Spectra and theory fits at effective coupling values quoted in the panels. **b**, Extracted bath temperatures of oscillator 2 and of the cavity.

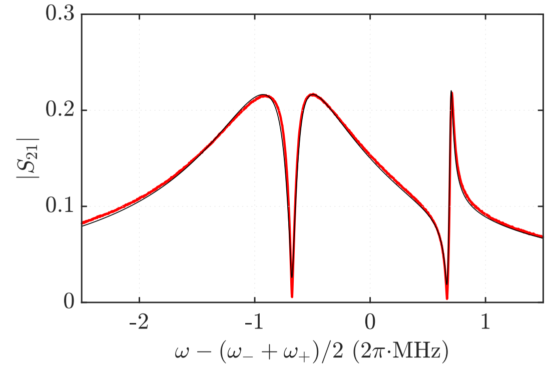


FIG. S6. *Cavity linear response, dataset* C. The black solid line is a theory prediction.

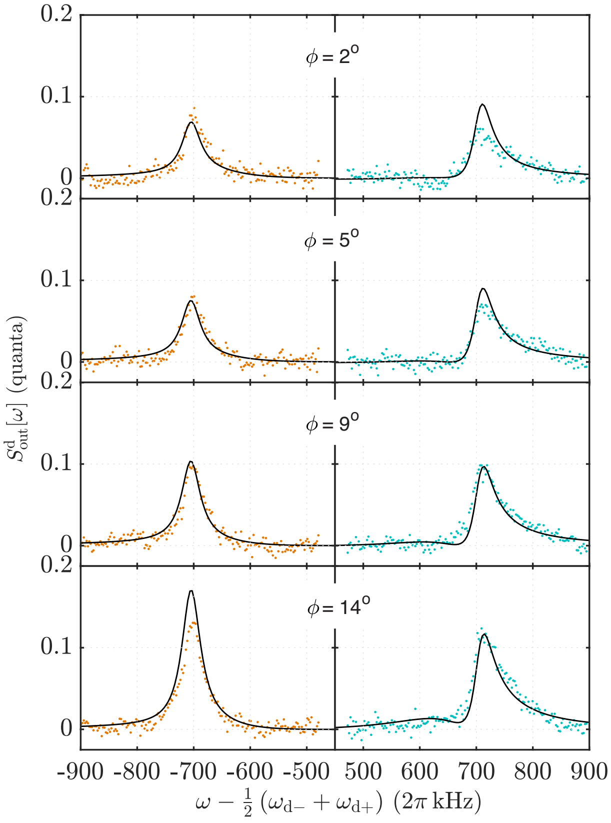


FIG. S7. *Probe data.* As Fig. 3 in main text, but for Dataset $D$, having a higher pump power $G_-/2\pi \simeq 332$ kHz.

Since there are plenty of parameters in a given measurement run, we prefer not to list them all in the main text. In Table I, we give a comprehensive list of all parameters pertaining to the displayed data. Because the experiment occurs at deep cryogenic temperatures $\ll \hbar\omega_c/k_B$, the external cavity noise $n_E^T$ is expected to be negligible. Here we can suppose that without any pump tones applied, the high-frequency modes thermalize close to the base temperature of the refrigerator. Under this condition, external noise that might nonetheless occur at higher pump powers would become treated essentially as internal cavity noise, appearing as a higher noise level.

TABLE I. *List of parameters for each dataset and graph.* The frequencies are given in linear frequencies (kHz). Dataset labels correspond to the respective panel labels (a...d) in Fig. 2 in main text. $\beta$ is the scaling factor of the probe area due to probe imbalance.

| dataset | | $G_-$ | $G_+$ | $g_-$ | $g_+$ | $n_1^{\mathrm{T}}$ | $n_2^{\mathrm{T}}$ | $n_{\mathrm{c}}^{\mathrm{T}}$ | $\Delta$ | $\bar{\delta}$ | $\Delta_{\mathrm{d}}$ | $\bar{\delta}_{\mathrm{d}}$ | $\beta$ |
|---|---|---|---|---|---|---|---|---|---|---|---|---|---|
| $A$ | red | 103 | 67 | - | - | 129 | 35 | 0.09 | 0.2 | $-5.8$ | - | - | - |
| | green | 103 | 74 | - | - | 140 | 35 | 0.11 | 0.2 | $-5.8$ | - | - | - |
| | orange | 103 | 82 | - | - | 124 | 36 | 0.15 | 0.2 | $-5.8$ | - | - | - |
| | cooling | 103 | 0 | - | - | 132 | - | 0.07 | 0 | $-10$ | - | - | - |
| $B$ | red | 201 | 135 | - | - | 152 | 54 | 0.24 | $-9.0$ | $-129$ | - | - | - |
| | orange | 201 | 135 | - | - | 167 | 63 | 0.24 | $-4.3$ | $-124$ | - | - | - |
| | green | 201 | 135 | - | - | 186 | 72 | 0.20 | 0 | $-120$ | - | - | - |
| | cooling | 201 | 0 | - | - | 117 | - | 0.17 | 0 | $-32$ | - | - | - |
| $C$ | red | 278 | 166 | 40 | 37.9 | 214 | 74 | 0.40 | 3.2 | 35 | 3.2 | $-639$ | 1.18 |
| | cooling | 278 | 0 | - | - | 96 | - | 0.28 | 0 | $-157$ | - | - | - |
| $D$ | red | 332 | 210 | 40 | 35 | 234 | 76 | 0.54 | 3.6 | 50 | 3.6 | $-674$ | 1.57 |
| | cooling | 332 | 0 | - | - | 138 | - | 0.43 | 0 | $-127$ | - | - | - |

## III. ERROR ANALYSIS

### A. Probe spectra

All the quoted error bars in this work are $2\sigma$ (95 %) confidence limits. In order to get the uncertainty estimate $\delta\langle X_+^2\rangle$ for the amount of two-mode squeezing in case of the 2-mode BAE detection, we use straightforward error analysis. Equation (S61b) used to determine $\langle X_+^2\rangle$ involves only calibrated parameters and the extracted peak area $n_{\mathrm{o}}$. We use uncorrelated error propagation to propagate the calibration uncertainties of $n_{\mathrm{o}}$, $\langle X_+^2\rangle_0$ and $\mathcal{N}$.

The error $\delta n_{\mathrm{o}}$ of the peak area below a given curve is obtained by comparing the experimental and theoretical $S^{\mathrm{d}}_{\mathrm{out,th}}[\omega]$ peak profiles as in Fig. 3 in the main text, more specifically, as the standard error of the residual:

$$\sigma_d = \frac{z}{\sqrt{N}}\sqrt{\frac{\sum_i^N \left[S^{\mathrm{d}}_{\mathrm{out}}(i) - S^{\mathrm{d}}_{\mathrm{out,th}}(i)\right]^2}{N}}\,. \tag{S73}$$

The sum is over frequency points $i$ in a single curve (total number $N$). The factor $z \simeq 2$ comes due to considering $2\sigma$ confidence. Instead of Eq. (S73), one can also fit Lorentzians to the peaks, and get the peak area uncertainties from the fit parameters. In the latter way, the errors are somewhat larger because the peaks deviate from a Lorentzian.

From Fig. S1b we obtain the uncertainty $\delta\langle X_+^2\rangle_0 \simeq 1.9$ as the error bar of the lowest-temperature data point. This error bar is larger than those of the surrounding points, but the size is reasonable given that it is roughly similar to the scatter seen in both panels in the low-temperature points. The scatter, presumably due to intermittent external disturbances such as building vibrations, is not directly captured in the statistical error bars from fitting the peak area.

From the power fit as in Fig. S2 we get $\delta\mathcal{N}/\mathcal{N} \simeq 2.2$ %. Among the contributions, the uncertainty of the peak area is clearly dominating for the final number $\delta\langle X_+^2\rangle$.

### B. Pump spectra

In the case of inferring parameters from the pump spectra, the uncertainty estimation is more involved. We can fit a theoretical expression of the pump spectrum to the data. This way we also obtain error estimates of the fit parameters, including the bath temperatures or decoherence rates that are the important figures determining the squeezing. However, we cannot use standard error propagation because the errors of the parameters will be correlated. In particular, what matters for the amount of two-mode squeezing or entanglement is not the decoherence rate of either mechanics individually, but the summed decoherence of the two mechanics put together, however, this is difficult to consider with error propagation.

We use Bayesian inference to estimate the system parameters from the pump spectra. Similar to standard least-squares fitting, we assume the data $S_{\mathrm{out}}$ is perfectly represented by the theoretical pump spectrum $S_{\mathrm{th}}(\theta_0)$ for some

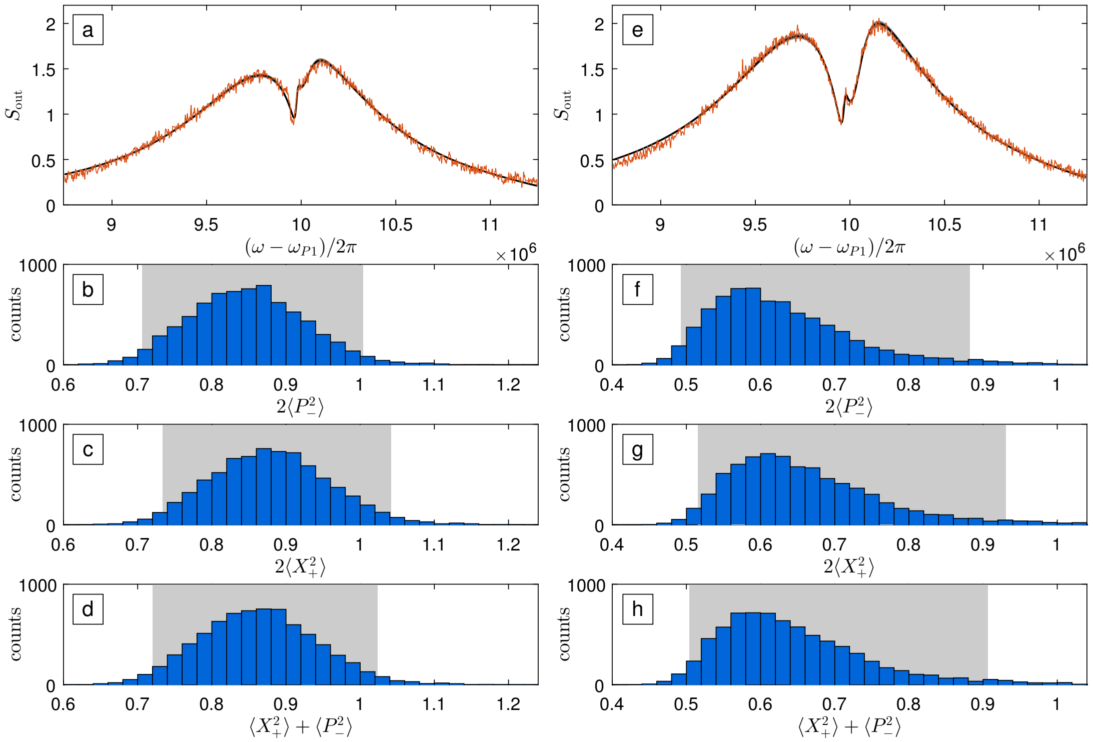


FIG. S8. Pump spectra and data analysis results for (a-d) dataset C and (e-h) dataset D. (a, e) Pump spectrum (red) with mean (black) and 95% confidence interval (gray shaded area) of the fitted theory model. (b-d, f-h) Histograms of the estimated distribution of quadrature occupations corresponding to panels a and e, respectively. Shaded area indicates 95% confidence interval.

true parameter vector $\theta_0$ plus white Gaussian noise with standard deviation $\sigma$. This is described by the likelihood function

$$p\left(S_{\rm out}|\theta\right)=\prod_i \frac{1}{\sqrt{2\pi}\sigma}\exp\left(-\frac{[S_{{\rm out},i}-S_{{\rm th},i}(\theta)]^2}{2\sigma^2}\right), \tag{S74}$$

where $\theta=\{G_-,G_+,n_1^{\rm T},n_2^{\rm T},n_{\rm c}^{\rm T},g_1,g_2/G_1,\delta_-,\delta_+,\kappa,\gamma_1,\gamma_2,\mathcal{A}\}$ is the vector of parameters to be estimated, and the index $i$ denotes the frequency bins of the spectrum.

We consider the Bayesian posterior distribution

$$p(\theta|S_{\rm out})=\frac{p(S_{\rm out}|\theta)p(\theta)}{Z}, \tag{S75}$$

where $p(\theta)$ is the prior distribution of the parameters $\theta$, and $Z$ is a normalization constant whose value is difficult to calculate but is not needed for the numerical method. For the prior $p(\theta)$ we choose a product of Gaussian distributions describing the calibration values and uncertainties of $\gamma_1$, $\gamma_2$, $\mathcal{A}$, $G_-$ and $g_1$. For all other parameters, we assume uniform (uninformed) prior distributions. We bound the thermal bath temperatures $n_1^{\rm T}>100$ and $n_2^{\rm T}>40$ from below to reflect the information from Figs. S4,S5 at high pump powers. All other parameters are bounded to be positive (except $\delta_-<0$) to avoid unphysical results. However, we do not place upper bounds on the parameters and hence have 8 free parameters in our analysis.

As the posterior distribution is difficult to calculate analytically, we use a numerical Monte Carlo method to generate a set of samples from $p(\theta|S_{\rm out})$. Specifically, we use an affine-invariant Markov chain Monte Carlo (MCMC) ensemble sampler [13] implemented in the open-source Python package *emcee* [14]. This method has recently been used for a similar problem in [15]. We initialize 150 walkers run them for 10000 steps to generate large number of pseudo-random parameter chains. We discard the first 5000 steps to ensure that the algorithm has converged to a steady state, and select a total of 7500 samples $\Theta$ from the remaining chain at regular intervals. The set $\Theta$ can be interpreted as samples of the distribution of parameters that agrees with the data and calibrations. In Fig. S8a,e we show the distribution of theory curves corresponding to $\Theta$ for the two datasets.

TABLE II. Mechanical quadrature occupations, expressed in quanta, derived from the estimated system parameters.

| Quadrature | Dataset C | Dataset D |
|---|---|---|
| $\langle X_+^2 \rangle$ | $0.44^{+0.08}_{-0.07}$ | $0.33^{+0.13}_{-0.07}$ |
| $\langle P_-^2 \rangle$ | $0.42^{+0.08}_{-0.07}$ | $0.31^{+0.13}_{-0.07}$ |
| $\langle X_-^2 \rangle$ | $5.8^{+1.7}_{-1.3}$ | $11.3^{+1.8}_{-1.7}$ |
| $\langle P_+^2 \rangle$ | $5.9^{+1.7}_{-1.3}$ | $11.4^{+1.8}_{-1.7}$ |
| $\langle X_+^2 \rangle + \langle P_-^2 \rangle$ | $0.86^{+0.16}_{-0.14}$ | $0.64^{+0.26}_{-0.14}$ |
| $p_{\rm ent}$ | 95.6% | 99.4% |

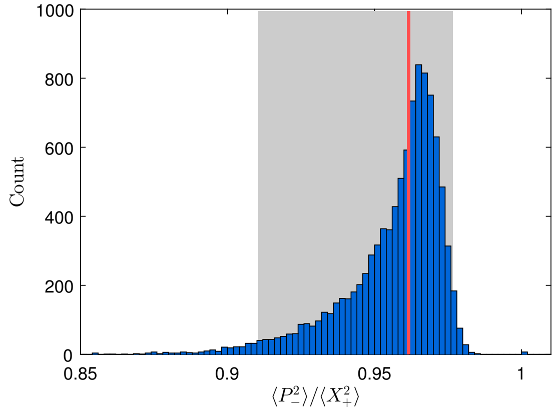


FIG. S9. Simulated ratio of quadrature variances for a wide range of system parameters, shown as a histogram. The vertical line and shaded area indicate the median and 95% confidence intervals, respectively.

Next, we evaluate $\langle X_+^2 \rangle$ and $\langle P_-^2 \rangle$ for each parameter vector in $\Theta$ numerically using Eq. (S45). This gives a distribution of quadrature occupations compatible with the pump spectrum and calibrations. Figure S8 shows histograms of the obtained quadrature occupations and the Duan quantity $\langle X_+^2 \rangle + \langle P_-^2 \rangle$, and the mean and 95% confidence intervals of the quadrature occupations are listed in table II. The probability of entanglement $p_{\rm ent}$ is calculated as the fraction of samples where the Duan quantity is below 1.

## C. Ratio of quadrature variances

Under our pumping scheme, the quadrature variances $\langle X_+^2 \rangle$ and $\langle P_-^2 \rangle$ are highly correlated and approximately equal. To quantify these correlations, we numerically evaluate the variances for a set of randomly generated system parameters, and for each parameter vector calculate the ratio $\langle P_-^2 \rangle / \langle X_+^2 \rangle$. The parameters are drawn from uniform distributions around the best fit values for dataset $C$. We emphasize that the parameter space included is much larger than the uncertainties obtained from fitting the pump spectra, and generously includes all calibration uncertainties.

As shown in Fig. S9, we find the ratio of variances is very narrowly distributed, and $\langle P_-^2 \rangle$ is consistently smaller than $\langle X_+^2 \rangle$. Hence, we can use this result as another consistency check on $\langle P_-^2 \rangle$ based on the direct measurement of $\langle X_+^2 \rangle$. We use the median and 95% confidence intervals $\langle P_-^2 \rangle / \langle X_+^2 \rangle = 0.962^{+0.015}_{-0.051}$ to obtain an estimate of $\langle P_-^2 \rangle$. For parameter values around the best fit to dataset $D$ we obtain similar results, $\langle P_-^2 \rangle / \langle X_+^2 \rangle = 0.955^{+0.019}_{-0.072}$.


[1] M. Aspelmeyer, T. J. Kippenberg, and F. Marquardt, *Rev. Mod. Phys.* **86**, 1391 (2014).
[2] Y.-D. Wang and A. A. Clerk, *Phys. Rev. Lett.* **110**, 253601 (2013).
[3] M. J. Woolley and A. A. Clerk, *Phys. Rev. A* **87**, 063846 (2013).
[4] M. J. Woolley and A. A. Clerk, *Phys. Rev. A* **89**, 063805 (2014).
[5] M. J. Woolley, A. C. Doherty, G. J. Milburn, and K. C. Schwab, *Phys. Rev. A* **78**, 062303 (2008).
[6] C. F. Ockeloen-Korppi, E. Damskägg, J.-M. Pirkkalainen, A. A. Clerk, M. J. Woolley, and M. A. Sillanpää, *Phys. Rev. Lett.* **117**, 140401 (2016).

[7] L. M. Duan, G. Giedke, J. I. Cirac, and P. Zoller, *Phys. Rev. Lett.* **84**, 2722 (2000).
[8] V. Giovannetti, S. Mancini, D. Vitali, and P. Tombesi, *Phys. Rev. A* **67**, 022320 (2003).
[9] H.-P. Breuer and F. Petrucionne, *The Theory of Open Quantum Systems*, Oxford University Press, 2002.
[10] C. W. Gardiner and P. Zoller, *Quantum Noise*, Springer, 2004.
[11] D. F. Walls and G. J. Milburn, *Quantum Optics*, Springer, 2008.
[12] J. D. Teufel, et al. Nature **475**, 359363 (2011).
[13] J. Goodman and J. Weare, *Communications in Applied Mathematics and Computational Science* **5**, 65 (2010).
[14] D. Foreman-Mackey, D. W. Hogg, D. Lang, J. Goodman, arXiv:1202.3665 (2012).
[15] E. E. Wollman, et al. *Science* **349**, 952 (2015).
